# Supplementary material for: Worst-Case Symbolic Constraints Analysis and Generalisation with Large Language Models
Source: arXiv:2506.08171 source file (2025-09-16)
Supplement: Supplementary file 2 [file appendix.tex]

% \section{Worst-Case Symbolic Constraint Generalisation with Large Language Models}
% \label{appendix:model_results}
% \renewcommand{\arraystretch}{1.2}
% \begin{table}[H]
% \caption{Symbolic Constraint Generalisation Accuracy (\%) per Model Across Trials.}
% \centering
% \small
% \begin{tabularx}{\textwidth}{>{\bfseries}l 
%     >{\raggedleft\arraybackslash}X 
%     >{\raggedleft\arraybackslash}X 
%     >{\raggedleft\arraybackslash}X 
%     >{\raggedleft\arraybackslash}X}
% \toprule
% Model & Trial 1 (\%) & Trial 2 (\%) & Trial 3 (\%) & Average (\%) \\
% \midrule
% gpt-4.1-nano-2025-04-14  & 33.98 & 38.15 & 34.87 & 35.67 \\
% gpt-4.1-mini-2025-04-14  & 39.94 & 38.15 & 41.58 & 39.89 \\
% gpt-4o-2024-11-20        & 43.52 & 42.03 & 44.11 & 43.22 \\
% gpt-3.5-turbo-0125       & 20.57 & 20.12 & 21.16 & 20.62 \\
% gpt-4o-mini-2024-07-18    & 30.10 & 31.00 & 28.91 & 30.00 \\
% gpt-4.1-2025-04-14       & 43.37 & 44.71 & 43.82 & \textbf{43.96} \\
% gpt-4-turbo-2024-04-09    & 40.83 & 40.24 & 40.54 & 40.54 \\
% \bottomrule
% \end{tabularx}
% \end{table}

\section{Motivating Example}
\label{appendix:motivating_example}

\section{Training Programs}
\label{appendix:post_training_programs}
\begin{table}[t]
\centering
\small
\caption{Overview of benchmark programs. The upper category comprises realistic programs including classical algorithms while the lower category contains programs sourced from the WISE benchmark suite.}
\begin{tabularx}{\textwidth}{@{} l X @{}}
\toprule
\textbf{Program} & \textbf{Description} \\
\midrule
\multicolumn{2}{@{}l}{\textbf{Custom / Authored}} \\[1ex]
\midrule
BinarySearch              & Classic divide-and-conquer search algorithm over sorted arrays. \\
BinarySearchTreeHeight    & Computes the height of a binary search tree built from symbolic integer insertions. \\
BubbleSort                & Elementary nested-loop sorting algorithm. \\
QuickSort                 & Recursive sorting algorithm using pivot-based partitioning. \\
MergeSort                 & Divide-and-conquer sorting algorithm with a merge step. \\
KnapsackSolver            & Recursive 0/1 knapsack dynamic programming variant. \\
NaiveFibonacci            & Exponential recursive Fibonacci computation. \\
TowerOfHanoi              & Recursive puzzle with exponential depth. \\
SubarraySumFinder         & Detects contiguous subarrays that sum to a symbolic target. \\
ArrayTwister              & Transforms an input array using modular arithmetic rules. \\
CaseFlipper               & Counts uppercase and lowercase characters in a symbolic character array. \\
Collatz                   & Simulates the Collatz sequence for symbolic inputs. \\
ComplexStateMachineParser & Parses a state machine with nested conditional transitions. \\
GreedyStepper             & Skips through an input array based on element parity. \\
RampUp                    & Triggers expensive computation only under a symbolic positivity constraint. \\
MazeSolver                & Solves a symbolic 2D maze via recursive backtracking. \\
DizzyRamp                 & Detects pattern changes in sequences and applies heavy cost on deviations. \\
\addlinespace
\midrule
\multicolumn{2}{@{}l}{\textbf{WISE Benchmark}} \\[1ex]
\midrule
BinaryTreeSearch          & Binary search tree insertion and search. \\
Dijkstra                  & Classic shortest path algorithm over a symbolic adjacency matrix. \\
SortedListInsert          & Sorted insertion into a linked list using symbolic keys. \\
\bottomrule
\end{tabularx}
\label{tab:benchmarks}
\end{table}
\begin{table}[H]
\label{tab:posttraining}
\centering
\caption{Overview of post-training programs. The upper section comprises synthetic programs designed for symbolic analysis, and the lower section contains code from Badger dataset.}
\small
\begin{tabularx}{\textwidth}{@{} l X @{}}
\toprule
\textbf{Program}      & \textbf{Description} \\
\midrule
\multicolumn{2}{@{}l}{\textbf{Custom / Authored}} \\[1ex]
\midrule
WeirdTimes            & Verifies each element equals the first element multiplied by its 1-based index; if so, executes a heavy loop. \\
WeirdNotFactor        & Ensures every non-initial element is an integer multiple of its predecessor (via floor/ceiling comparisons) before heavy computation. \\
WeirdLoopMean         & Computes the array mean and uses it to set the iteration count of an intensive multiplication loop. \\
WeirdHundred          & Checks elements against a 100 threshold, conditioned on the first element (1 or 0), and then performs heavy computation. \\
WeirdFibonacci        & Validates a Fibonacci-like progression (each element equals the sum of the two previous ones) before heavy computation. \\
WeirdConstDiff        & Confirms constant differences between consecutive elements (arithmetic progression) prior to heavy processing. \\
SimpleUnique          & Verifies all characters in an array are unique before triggering a heavy loop. \\
SimpleTrueFalse       & Ensures an alternating boolean pattern (false at even, true at odd indices) before heavy computation. \\
SimpleSymmetric       & Checks matrix symmetry by comparing mirrored elements; if valid, executes a heavy loop. \\
SimpleSignFlip        & Requires adjacent elements to be equal at even indices and strictly increasing at odd indices, then triggers heavy computation. \\
SimpleEveryThird      & Checks that every third element meets a specified condition before heavy processing. \\
SimpleAscendingLast   & Verifies that the last element is strictly greater than its predecessor before heavy computation. \\
SameString            & Confirms all characters in a string are identical, then executes a heavy loop. \\
SameOnlyThird         & Applies a condition solely to the third element; triggers heavy computation if satisfied. \\
SameLowercase         & Ensures every character in the string is lowercase before heavy processing. \\
SameHundred           & Verifies all elements equal 100, then triggers heavy computation. \\
ComplexPalindrome     & Checks if an input sequence is palindromic before executing a heavy loop. \\
ComplexOddsEvens      & Validates that odd- and even-indexed elements satisfy distinct conditions before heavy computation. \\
ComplexMidPeak        & Confirms that the middle segment of the array forms a peak pattern prior to heavy processing. \\
ComplexHalfEqual      & Verifies that the first half of the array equals the second half before heavy computation. \\
\midrule
\multicolumn{2}{@{}l}{\textbf{Badger}} \\[1ex]
\midrule
BadgerHash            & Implements a symbolic hash routine and validates its output before heavy computation. \\
BadgerPassword        & Processes a symbolic password transformation, triggering heavy computation upon validation. \\
BadgerUsername        & Verifies a symbolic username against complexity requirements and then executes a heavy loop. \\
\bottomrule
\end{tabularx}
\end{table}

\section{Benchmark Programs}
\label{appendix:benchmark_programs}

\section{Quick Sort Example Prompts for Tiered Evaluation}
\label{appendix:prompts}

The examples below illustrate a tiered approach for evaluating generalisation performance using \textbf{jump size} as a measure of difficulty. At each tier, the model is presented with a set of example constraints for smaller input sizes and asked to extrapolate the corresponding constraint for a larger target size \(N\). 

We define jump size as the difference between the largest example input and the target \(N\), and classify it into three categories:
\begin{itemize}
    \item \textbf{Small jump:} \(\leq 5\)
    \item \textbf{Medium jump:} \(6 \leq \text{jump} \leq 15\)
    \item \textbf{Large jump:} \(> 15\)
\end{itemize}

Each tier increases in complexity, requiring models to perform progressively more challenging forms of pattern extrapolation, up to a maximum of \(N = 30\).

\paragraph{Small Tier (Target \(\mathbf{N=4}\))}
\noindent
This tier tests minimal leaps (e.g.\ from \(N=3\) to \(N=4\)):

\noindent\rule{\linewidth}{0.4pt}
\textbf{Prompt:}
\begin{lstlisting}
Given the following examples of constraints for increasing input sizes:
N=1: None
N=2: (assert  ( <=  in0 in1))
N=3: (assert (and (and  ( <=  in0 in2)  ( <=  in1 in2))  ( <=  in0 in1)))
What is the constraint for N=4?
\end{lstlisting}
\rule{\linewidth}{0.4pt}

\paragraph{Medium Tier (Target \(\mathbf{N=10}\))}
\noindent
Here, we move from smaller constraints (e.g.\ \(N=3, 5\)) to a moderate jump at \(N=11\):

\noindent\rule{\linewidth}{0.4pt}
\textbf{Prompt:}
\begin{lstlisting}
Given the following examples of constraints for increasing input sizes:
N=1: None
N=3: (assert (and (and  ( <=  in0 in2)  ( <=  in1 in2))  ( <=  in0 in1)))
N=5: (assert (and (and (and (and (and (and (and (and (and  ( <=  in0 in4)  ( <=  in1 in4))  ( <=  in2 in4))  ( <=  in3 in4))  ( <=  in0 in3))  ( <=  in1 in3))  ( <=  in2 in3))  ( <=  in0 in2))  ( <=  in1 in2))  ( <=  in0 in1)))
What is the constraint for N=11?
\end{lstlisting}
\rule{\linewidth}{0.4pt}

\paragraph{Large Tier (Target \(\mathbf{N=30}\))}
\noindent
A “hard” prompt might jump from much smaller examples (e.g.\ \(N=1,3,4, 8\)) all the way to \(N=30\), demonstrating maximal extrapolation demands:

\noindent\rule{\linewidth}{0.4pt}
\textbf{Prompt:}
\begin{lstlisting}
Given the following examples of constraints for increasing input sizes:
N=1: None
N=3: (assert (and (and  ( <=  in0 in2)  ( <=  in1 in2))  ( <=  in0 in1)))
N=4: (assert (and (and (and (and (and  ( <=  in0 in3)  ( <=  in1 in3))  ( <=  in2 in3))  ( <=  in0 in2))  ( <=  in1 in2))  ( <=  in0 in1)))
N=8: (assert (and (and (and (and (and (and (and (and (and (and (and (and (and (and (and (and (and (and (and (and (and (and (and (and (and (and (and  ( <=  in0 in7)  ( <=  in1 in7))  ( <=  in2 in7))  ( <=  in3 in7))  ( <=  in4 in7))  ( <=  in5 in7))  ( <=  in6 in7))  ( <=  in0 in6))  ( <=  in1 in6))  ( <=  in2 in6))  ( <=  in3 in6))  ( <=  in4 in6))  ( <=  in5 in6))  ( <=  in0 in5))  ( <=  in1 in5))  ( <=  in2 in5))  ( <=  in3 in5))  ( <=  in4 in5))  ( <=  in0 in4))  ( <=  in1 in4))  ( <=  in2 in4))  ( <=  in3 in4))  ( <=  in0 in3))  ( <=  in1 in3))  ( <=  in2 in3))  ( <=  in0 in2))  ( <=  in1 in2))  ( <=  in0 in1)))
What is the constraint for N=30?
\end{lstlisting}
\rule{\linewidth}{0.4pt}

\medskip

\noindent

By structuring tiers to vary the jump size, we provide a more nuanced measure of difficulty. Models must exhibit not only incremental pattern extension but also robust extrapolation over substantial gaps, all while remaining within a verifiable domain \(\mathbf{N \le 30}\).

\section{Benchmark Profile}
\label{appendix:benchmark_profile}

We provide a comprehensive overview of the statistical properties of our benchmark dataset, which comprises 671 instances. In this section, we present detailed metrics on token counts for both questions and answers, the distribution of instances across defined difficulty tiers, characteristics of answer texts, and problem-specific parameters such as target values and the number of example constraints.

\subsection{Token Statistics}

To provide insight into the textual complexity of our benchmark dataset, we computed a range of token-based metrics for both questions and answers. These metrics—including minimum, maximum, average, median, standard deviation, and various percentiles—are instrumental in assessing the size, variability, and distribution of tokens in our dataset. We leverage the \texttt{Qwen/Qwen2.5-3B} tokenizer for these metrics.

\begin{table}[H]
  \centering
  \caption{Token Statistics for Questions and Answers}
  \label{tab:combined_token_stats}
  \begin{tabularx}{\textwidth}{l >{\raggedleft\arraybackslash}X >{\raggedleft\arraybackslash}X}
    \toprule
    \textbf{Statistic} & \textbf{Questions} & \textbf{Answers} \\ \midrule
    Minimum Token Count & 117   & 27 \\
    Maximum Token Count & 4086  & 14,476 \\
    Average Token Count & 1684.28 & 993.61 \\
    Median Token Count  & 1521  & 493 \\
    Standard Deviation of Token Count & 1146.45 & 1349.36 \\
    Total Token Count   & 1,130,153 & 666,709 \\
    25th Percentile Token Count & 645   & 209 \\
    50th Percentile Token Count & 1521  & 493 \\
    75th Percentile Token Count & 2594.5 & 1196 \\
    90th Percentile Token Count & 3371  & 2659 \\
    95th Percentile Token Count & 3767.5 & 3590 \\
    99th Percentile Token Count & 4056.6 & 5780.20 \\
    \bottomrule
  \end{tabularx}
\end{table}

\subsection{Tier Statistics}

We present the breakdown of examples across difficulty tiers, defined by the \emph{jump size} metric (see \autoref{subsec: constraint curation}. We calculated the average token counts for questions and answers in each tier.

\begin{table}[H]
  \centering
  \caption{Tier Statistics of the Benchmark Dataset}
  \label{tab:tier_stats}
  \begin{tabularx}{\textwidth}{l*{4}{>{\centering\arraybackslash}X}}
    \toprule
    \textbf{Difficulty Tier} & \textbf{Example Count} & \textbf{Percentage of Total (\%)} & \textbf{Average Question Token Count} & \textbf{Average Answer Token Count} \\
    \midrule
    Small  & 333 & 49.63 & 1797.49 & 810.50 \\
    Medium & 333 & 49.63 & 1579.74 & 1161.27 \\
    Large  & 5   & 0.75  & 1106.80 & 2021.60 \\
    \bottomrule
  \end{tabularx}
\end{table}

\subsection{Problem Parameters}

\autoref{tab:target_n_stats} details the distribution of target \(N\) values, and \autoref{tab:example_counts_stats} provides statistics on the number of example constraints per problem.

\begin{table}[H]
  \centering
  \caption{Target \(N\) Value Distribution}
  \label{tab:target_n_stats}
  \begin{tabularx}{\textwidth}{l >{\raggedleft\arraybackslash}X}
    \toprule
    \textbf{Statistic} & \textbf{Value} \\ \midrule
    Minimum Target Value & 5 \\
    Maximum Target Value & 30 \\
    Average Target Value & 19.86 \\
    Median Target Value  & 20 \\
    Unique Target Values & \multicolumn{1}{>{\raggedleft\arraybackslash}X}{%
      \parbox[t]{0.6\textwidth}{\raggedleft
        5 \quad 7 \quad 8 \quad 9 \quad 10\\[3pt]
        11 \quad 12 \quad 13 \quad 14 \quad 15\\[3pt]
        16 \quad 17 \quad 18 \quad 19 \quad 20\\[3pt]
        21 \quad 22 \quad 23 \quad 24 \quad 25\\[3pt]
        26 \quad 27 \quad 28 \quad 29 \quad 30
      }
    } \\
    \bottomrule
  \end{tabularx}
\end{table}

\begin{table}[H]
  \centering
  \caption{Example Constraint Count Statistics per Problem}
  \label{tab:example_counts_stats}
  \begin{tabularx}{\textwidth}{l >{\raggedleft\arraybackslash}X}
    \toprule
    \textbf{Statistic} & \textbf{Value} \\ \midrule
    Minimum Number of Constraints & 3 \\
    Maximum Number of Constraints & 18 \\
    Average Number of Constraints & 6.67 \\
    Median Number of Constraints  & 6 \\
    \bottomrule
  \end{tabularx}
\end{table}

\subsection{Visualisations}

The following figures provide visual representations of key distributions in the dataset.

\begin{figure}[H]
  \centering
  \includegraphics[width=0.8\textwidth]{figures/example_count_distribution.png}
  \caption{Histogram of Example Constraint Counts per Problem.}
  \label{fig:example_count_distribution}
\end{figure}

\begin{figure}[H]
  \centering
  \includegraphics[width=0.8\textwidth]{figures/target_n_distribution.png}
  \caption{Distribution of Target \(N\) Values.}
  \label{fig:target_n_distribution}
\end{figure}

\begin{figure}[H]
  \centering
  \includegraphics[width=0.8\textwidth]{figures/tier_distribution.png}
  \caption{Distribution of Examples Across Difficulty Tiers.}
  \label{fig:tier_distribution}
\end{figure}

\begin{figure}[H]
  \centering
  \includegraphics[width=0.8\textwidth]{figures/token_by_tier.png}
  \caption{Average Token Counts for Questions and Answers by Difficulty Tier.}
  \label{fig:token_by_tier}
\end{figure}

\begin{figure}[H]
  \centering
  \includegraphics[width=0.8\textwidth]{figures/token_distributions.png}
  \caption{Histograms of Token Count Distributions for Questions and Answers.}
  \label{fig:token_distributions}
\end{figure}
